# Supplementary material for: Fusing Higher-order Features in Graph Neural Networks for Skeleton-based Action Recognition
Source: arXiv:2105.01563 source file (2022-08-23)
Supplement: Supplementary file 1 [file appendix.tex]

We provide the improvement of accuracy by angular encoding for each class. The results for the static domain are in  \autoref{table:static_complete_action_imp_1} and  \autoref{table:static_complete_action_imp_2}. The ones for the velocity domain are in \autoref{table:velocity_complete_action_imp_1} and \autoref{table:velocity_complete_action_imp_2}.

\begin{table*}[t]
\centering
% \vspace{-2mm}
\caption{Static: First Half. }
\resizebox{\textwidth}{!}{
\begin{tabular}{l|rc|rrc}
\toprule 
%\rowcolor{Gray}
 & \multicolumn{2}{c|}{\textbf{Joint}} & \multicolumn{3}{c}{\textbf{Concatenation: Joint + Angular}} \\
\cline{2-3}\cline{4-6}
%\rowcolor{Gray}
\multirow{-2}{*}{\textbf{Action}} & Acc (\%) & Similar Action & Acc (\%) & Acc$\uparrow$ (\%) & Similar Action \\ 
\midrule 
% \rowcolor{Gray!30}
make victory sign & 18.48 & thumb up   & 53.04 & 34.57 & make ok sign   \\
staple book & 26.67 & staple book   & 37.13 & 10.46 & cutting paper (using scissors)   \\
writing & 28.41 & typing on a keyboard   & 48.90 & 20.49 & typing on a keyboard   \\
counting money & 48.47 & play magic cube   & 52.98 & 4.51 & play magic cube   \\
playing with phone/tablet & 48.82 & play magic cube   & 59.64 & 10.82 & writing   \\
wield knife towards other person & 49.52 & hit other person with something   & 62.50 & 12.98 & hit other person with something   \\
% make ok sign & 54.48 & make victory sign   & 48.52 & -5.96 & make victory sign   \\
blow nose & 55.35 & yawn   & 59.65 & 4.30 & yawn   \\
fold paper & 56.57 & ball up paper   & 62.78 & 6.22 & counting money   \\
reading & 58.34 & cutting paper (using scissors)   & 64.10 & 5.76 & writing   \\
thumb up & 58.65 & make victory sign   & 72.35 & 13.70 & make victory sign   \\
yawn & 59.00 & hush (quite)   & 67.65 & 8.65 & hush (quite)   \\
snapping fingers & 59.10 & shake fist   & 65.51 & 6.40 & make victory sign   \\
open a box & 59.98 & fold paper   & 71.60 & 11.63 & open bottle   \\
% play magic cube & 62.81 & counting money   & 59.97 & -2.85 & playing with phone/tablet   \\
% cutting nails & 63.32 & playing with phone/tablet   & 63.09 & -0.23 & playing with phone/tablet   \\
pointing to something with finger & 64.58 & taking a selfie   & 79.71 & 15.13 & taking a selfie   \\
sneeze/cough & 64.58 & touch head (headache)   & 71.74 & 7.16 & touch head (headache)   \\
apply cream on hand back & 67.82 & open bottle   & 72.30 & 4.48 & rub two hands together   \\
cutting paper (using scissors) & 68.28 & staple book   & 70.16 & 1.87 & staple book   \\
typing on a keyboard & 68.45 & cutting paper (using scissors)   & 69.09 & 0.64 & writing   \\
% hit other person with something & 69.09 & wield knife towards other person   & 62.26 & -6.83 & wield knife towards other person   \\
hush (quite) & 69.16 & yawn   & 72.08 & 2.92 & yawn   \\
ball up paper & 69.26 & fold paper   & 71.30 & 2.04 & fold paper   \\
eat meal/snack" & 69.55 & brushing teeth   & 71.27 & 1.73 & brushing teeth   \\
wear a shoe & 70.43 & take off a shoe   & 85.35 & 14.92 & take off a shoe   \\
% shoot at other person with a gun & 70.83 & take a photo of other person   & 70.09 & -0.74 & point finger at the other person   \\
take off a shoe & 70.90 & wear a shoe   & 81.75 & 10.85 & wear a shoe   \\
punching/slapping other person & 72.36 & hit other person with something   & 82.85 & 10.49 & hit other person with something   \\
open bottle & 73.17 & play magic cube   & 73.82 & 0.65 & open a box   \\
put something into a bag & 73.26 & take something out of a bag   & 79.13 & 5.87 & take something out of a bag   \\
shake fist & 74.69 & hand waving   & 76.39 & 1.69 & snapping fingers   \\
touch head (headache) & 75.45 & drink water   & 82.25 & 6.80 & touch neck (neckache)   \\
thumb down & 75.52 & thumb up   & 80.87 & 5.35 & pointing to something with finger   \\
sniff (smell) & 76.04 & blow nose   & 81.04 & 5.00 & blow nose   \\
make a phone call/answer phone & 80.09 & reading   & 87.64 & 7.55 & playing with phone/tablet   \\
% flick hair & 80.39 & blow nose   & 80.00 & -0.39 & brushing hair   \\
% throw up cap/hat & 80.50 & shoot at the basket   & 78.01 & -2.49 & toss a coin   \\
apply cream on face & 80.71 & wipe face   & 83.10 & 2.39 & wipe face   \\
rub two hands together & 80.88 & clapping   & 82.61 & 1.72 & apply cream on hand back   \\
touch neck (neckache) & 80.88 & drink water   & 87.32 & 6.43 & flick hair   \\
nausea or vomiting condition & 81.18 & sneeze/cough   & 84.73 & 3.55 & touch chest (stomachache/heart pain)   \\
% shoot at the basket & 81.34 & throw   & 80.24 & -1.10 & throw   \\
drink water & 81.48 & brushing teeth   & 83.94 & 2.46 & brushing teeth   \\
move heavy objects & 81.57 & carry something with other person   & 86.09 & 4.52 & carry something with other person   \\
take something out of a bag & 81.64 & put something into a bag   & 84.90 & 3.26 & put something into a bag   \\
brushing teeth & 81.78 & drink water   & 87.55 & 5.76 & touch head (headache)   \\
drop & 81.91 & staple book   & 85.82 & 3.91 & tear up paper   \\
put the palms together & 81.97 & cross hands in front (say stop)   & 92.75 & 10.78 & sniff (smell)   \\
point finger at the other person & 81.97 & pat on back of other person   & 88.77 & 6.80 & pat on back of other person   \\
use a fan (with hand or paper)/feeling warm & 82.27 & hand waving   & 89.82 & 7.55 & shake fist   \\
check time (from watch) & 82.33 & open bottle   & 90.58 & 8.25 & put the palms together   \\
% clapping & 82.52 & rub two hands together   & 81.69 & -0.83 & rub two hands together   \\
support somebody with hand & 82.65 & follow other person   & 88.70 & 6.04 & knock over other person (hit with body)   \\
take off headphone & 82.92 & take off glasses   & 86.40 & 3.47 & take off glasses   \\
tennis bat swing & 83.15 & throw up cap/hat   & 83.45 & 0.30 & throw up cap/hat   \\
take off glasses & 83.67 & take off headphone   & 93.07 & 9.39 & take off headphone   \\
knock over other person (hit with body) & 83.72 & whisper in other person’s ear   & 88.89 & 5.17 & whisper in other person’s ear   \\
wipe face & 83.78 & brushing hair   & 87.68 & 3.90 & brushing hair   \\
reach into pocket & 84.04 & touch back (backache)   & 85.40 & 1.36 & typing on a keyboard   \\
\bottomrule 
\end{tabular}
}
\label{table:static_complete_action_imp_1}
\end{table*}

\begin{table*}[t]
% Second Half 
\caption{Static: Second Half. }
\resizebox{\textwidth}{!}{
\begin{tabular}{l|rc|rrc}
\toprule 
%\rowcolor{Gray}
 & \multicolumn{2}{c|}{\textbf{Joint}} & \multicolumn{3}{c}{\textbf{Concatenation: Joint + Angular}} \\
\cline{2-3}\cline{4-6}
%\rowcolor{Gray}
\multirow{-2}{*}{\textbf{Action}} & Acc (\%) & Similar Action & Acc (\%) & Acc$\uparrow$ (\%) & Similar Action \\ 
\midrule 
% \rowcolor{Gray!30}
put on headphone & 84.20 & wear on glasses   & 87.52 & 3.32 & take off headphone   \\
throw & 84.82 & wear jacket   & 91.27 & 6.45 & stretch oneself   \\
side kick & 84.89 & kicking something   & 90.77 & 5.88 & kicking something   \\
tear up paper & 84.98 & fold paper   & 88.19 & 3.21 & wear jacket   \\
wear on glasses & 85.08 & drink water   & 88.28 & 3.20 & eat meal/snack"   \\
nod head/bow & 85.23 & nausea or vomiting condition   & 94.93 & 9.70 & nausea or vomiting condition   \\
kicking other person & 85.59 & step on foot   & 91.30 & 5.71 & punching/slapping other person   \\
% grab other person’s stuff & 85.78 & hit other person with something   & 85.57 & -0.22 & touch other person's pocket   \\
touch chest (stomachache/heart pain) & 85.96 & touch back (backache)   & 91.30 & 5.35 & touch back (backache)   \\
toss a coin & 86.09 & throw up cap/hat   & 89.01 & 2.92 & make victory sign   \\
exchange things with other person & 86.48 & giving something to other person   & 89.04 & 2.57 & giving something to other person   \\
step on foot & 86.65 & kicking other person   & 89.39 & 2.74 & kicking other person   \\
cross toe touch & 86.80 & move heavy objects   & 89.90 & 3.09 & move heavy objects   \\
brushing hair & 86.91 & wipe face   & 88.64 & 1.73 & touch head (headache)   \\
taking a selfie & 87.04 & reading   & 90.22 & 3.17 & pointing to something with finger   \\
put on bag & 87.35 & take something out of a bag   & 93.91 & 6.57 & wear jacket   \\
take off bag & 87.72 & tennis bat swing   & 92.36 & 4.65 & take off jacket   \\
whisper in other person’s ear & 87.87 & knock over other person (hit with body)   & 88.87 & 1.00 & knock over other person (hit with body)   \\
% giving something to other person & 88.49 & exchange things with other person   & 87.68 & -0.81 & exchange things with other person   \\
cross arms & 88.74 & cross hands in front (say stop)   & 94.09 & 5.35 & put the palms together   \\
stretch oneself & 88.93 & hands up (both hands)   & 93.06 & 4.13 & hands up (both hands)   \\
cheer up & 89.15 & hand waving   & 90.51 & 1.36 & use a fan (with hand or paper)/feeling warm   \\
put on a hat/cap & 89.44 & wear on glasses   & 94.85 & 5.41 & wear on glasses   \\
salute & 89.58 & shake head   & 92.03 & 2.45 & shake head   \\
hand waving & 89.88 & use a fan (with hand or paper)/feeling warm   & 90.15 & 0.27 & shake fist   \\
% pat on back of other person & 90.30 & point finger at the other person   & 88.77 & -1.54 & point finger at the other person   \\
take a photo of other person & 90.32 & shoot at other person with a gun   & 94.27 & 3.95 & shoot at other person with a gun   \\
hands up (both hands) & 90.81 & stretch oneself   & 94.25 & 3.44 & stretch oneself   \\
take off a hat/cap & 90.94 & throw up cap/hat   & 96.70 & 5.76 & apply cream on face   \\
juggling table tennis balls & 91.15 & toss a coin   & 95.81 & 4.66 & snapping fingers   \\
falling & 91.36 & move heavy objects   & 93.82 & 2.45 & staggering   \\
touch other person's pocket & 91.36 & giving something to other person   & 94.91 & 3.55 & pat on back of other person   \\
touch back (backache) & 91.39 & touch chest (stomachache/heart pain)   & 94.20 & 2.81 & touch chest (stomachache/heart pain)   \\
sitting down & 91.67 & falling   & 94.51 & 2.83 & kicking something   \\
standing up (from sitting position) & 91.67 & take off a shoe   & 95.97 & 4.30 & nausea or vomiting condition   \\
shake head & 91.73 & touch back (backache)   & 92.00 & 0.27 & make victory sign   \\
staggering & 91.75 & walking apart from each other   & 98.91 & 7.16 & follow other person   \\
butt kicks (kick backward) & 91.86 & side kick   & 94.43 & 2.57 & side kick   \\
% pickup & 92.45 & take off a shoe   & 92.00 & -0.45 & take off a shoe   \\
squat down & 92.73 & sitting down   & 96.86 & 4.14 & falling   \\
cross hands in front (say stop) & 92.84 & taking a selfie   & 93.12 & 0.28 & put the palms together   \\
bounce ball & 92.86 & running on the spot   & 94.21 & 1.35 & finger-guessing game (playing rock-paper-scissors)   \\
finger-guessing game (playing rock-paper-scissors) & 92.92 & shake fist   & 94.97 & 2.04 & shake fist   \\
kicking something & 93.20 & side kick   & 94.20 & 1.00 & staggering   \\
hopping (one foot jumping) & 93.55 & staggering   & 96.00 & 2.45 & kicking something   \\
take off jacket & 93.93 & tear up paper   & 96.38 & 2.45 & wear jacket   \\
wear jacket & 94.64 & tear up paper   & 98.91 & 4.27 & put on bag   \\
running on the spot & 95.17 & hopping (one foot jumping)   & 97.39 & 2.22 & butt kicks (kick backward)   \\
high-five & 95.18 & hit other person with something   & 97.05 & 1.87 & giving something to other person   \\
% carry something with other person & 95.18 & move heavy objects   & 93.58 & -1.60 & support somebody with hand   \\
walking apart from each other & 95.38 & walking towards each other   & 96.74 & 1.36 & walking towards each other   \\
arm swings & 95.52 & arm circles   & 98.61 & 3.09 & arm circles   \\
pushing other person & 95.74 & hugging other person   & 96.01 & 0.28 & walking apart from each other   \\
% handshaking & 95.74 & shake head   & 95.29 & -0.45 & giving something to other person   \\
follow other person & 95.88 & walking apart from each other   & 96.01 & 0.13 & walking apart from each other   \\
arm circles & 96.22 & stretch oneself   & 98.96 & 2.74 & stretch oneself   \\
cheers and drink & 96.22 & take a photo of other person   & 97.57 & 1.35 & drink water   \\
hugging other person & 96.45 & falling   & 97.81 & 1.36 & falling   \\
jump up & 96.83 & running on the spot   & 98.19 & 1.36 & kicking something   \\
walking towards each other & 97.17 & follow other person   & 99.27 & 2.10 & staggering   \\
\bottomrule 
\end{tabular}
}
\label{table:static_complete_action_imp_2}
\end{table*}

% % Velocity 

\begin{table*}[t]
\centering
% \vspace{-2mm}
\caption{Velocity: First Half. }
\resizebox{\textwidth}{!}{
\begin{tabular}{l|rc|rrc}
\toprule 
%\rowcolor{Gray}
 & \multicolumn{2}{c|}{\textbf{Joint}} & \multicolumn{3}{c}{\textbf{Concatenation: Joint + Angular}} \\
\cline{2-3}\cline{4-6}
%\rowcolor{Gray}
\multirow{-2}{*}{\textbf{Action}} & Acc (\%) & Similar Action & Acc (\%) & Acc$\uparrow$ (\%) & Similar Action \\ 
\midrule 
% \rowcolor{Gray!30} 
make ok sign & 27.17 & make ok sign   & 46.78 & 19.61 & make victory sign   \\
cutting paper (using scissors) & 27.27 & staple book   & 60.38 & 33.11 & staple book   \\
staple book & 30.17 & cutting paper (using scissors)   & 31.52 & 1.35 & staple book   \\
playing with phone/tablet & 39.73 & writing   & 64.00 & 24.27 & typing on a keyboard   \\
play magic cube & 45.50 & counting money   & 65.21 & 19.71 & counting money   \\
% make victory sign & 46.48 & make ok sign   & 40.52 & -5.96 & make ok sign   \\
reading & 48.82 & writing   & 58.61 & 9.79 & writing   \\
counting money & 49.00 & play magic cube   & 50.70 & 1.70 & play magic cube   \\
blow nose & 52.04 & yawn   & 62.96 & 10.91 & yawn   \\
thumb up & 53.43 & make victory sign   & 63.30 & 9.87 & make victory sign   \\
cutting nails & 54.89 & writing   & 58.17 & 3.28 & playing with phone/tablet   \\
hit other person with something & 55.35 & wield knife towards other person   & 58.43 & 3.09 & wield knife towards other person   \\
typing on a keyboard & 56.45 & writing   & 66.18 & 9.73 & writing   \\
open a box & 56.84 & open bottle   & 65.16 & 8.32 & open bottle   \\
shoot at other person with a gun & 57.78 & point finger at the other person   & 63.83 & 6.04 & point finger at the other person   \\
fold paper & 57.96 & ball up paper   & 65.91 & 7.96 & ball up paper   \\
yawn & 58.30 & hush (quite)   & 64.00 & 5.70 & hush (quite)   \\
wield knife towards other person & 59.76 & hit other person with something   & 61.28 & 1.52 & hit other person with something   \\
pointing to something with finger & 60.96 & taking a selfie   & 72.46 & 11.51 & taking a selfie   \\
snapping fingers & 63.46 & shake fist   & 65.68 & 2.22 & shake fist   \\
open bottle & 64.10 & open a box   & 73.65 & 9.55 & play magic cube   \\
sneeze/cough & 65.30 & touch head (headache)   & 68.12 & 2.81 & touch head (headache)   \\
touch head (headache) & 65.67 & brushing teeth   & 73.91 & 8.25 & brushing teeth   \\
hush (quite) & 68.46 & yawn   & 74.17 & 5.71 & blow nose   \\
% writing & 69.96 & typing on a keyboard   & 48.90 & -21.06 & typing on a keyboard   \\
% ball up paper & 71.70 & counting money   & 70.96 & -0.74 & play magic cube   \\
touch neck (neckache) & 71.83 & touch head (headache)   & 82.25 & 10.42 & touch head (headache)   \\
flick hair & 71.87 & blow nose   & 77.74 & 5.87 & brushing hair   \\
% eat meal/snack" & 72.09 & brushing teeth   & 69.09 & -3.00 & brushing teeth   \\
drink water & 72.72 & brushing teeth   & 85.77 & 13.04 & brushing teeth   \\
shoot at the basket & 73.65 & throw   & 82.34 & 8.69 & hands up (both hands)   \\
put something into a bag & 73.78 & take something out of a bag   & 78.09 & 4.30 & take something out of a bag   \\
shake fist & 74.17 & hand waving   & 76.22 & 2.04 & hand waving   \\
throw up cap/hat & 74.57 & toss a coin   & 79.23 & 4.66 & toss a coin   \\
wipe face & 75.09 & touch head (headache)   & 87.68 & 12.59 & touch head (headache)   \\
nausea or vomiting condition & 75.36 & touch chest (stomachache/heart pain)   & 80.36 & 5.00 & touch chest (stomachache/heart pain)   \\
% sniff (smell) & 76.22 & make victory sign   & 73.39 & -2.83 & hush (quite)   \\
take off a shoe & 76.74 & wear a shoe   & 83.21 & 6.47 & wear a shoe   \\
taking a selfie & 77.26 & drink water   & 83.33 & 6.07 & pointing to something with finger   \\
knock over other person (hit with body) & 77.65 & wield knife towards other person   & 82.12 & 4.47 & wield knife towards other person   \\
% clapping & 78.12 & rub two hands together   & 78.02 & -0.10 & rub two hands together   \\
take something out of a bag & 78.17 & put something into a bag   & 82.47 & 4.30 & put something into a bag   \\
% apply cream on hand back & 78.27 & rub two hands together   & 76.66 & -1.61 & rub two hands together   \\
wear a shoe & 78.49 & take off a shoe   & 81.69 & 3.20 & take off a shoe   \\
take off headphone & 78.68 & take off glasses   & 84.98 & 6.30 & take off glasses   \\
make a phone call/answer phone & 79.00 & drink water   & 81.82 & 2.82 & playing with phone/tablet   \\
thumb down & 79.87 & thumb up   & 82.78 & 2.91 & thumb up   \\
support somebody with hand & 79.87 & follow other person   & 82.26 & 2.39 & follow other person   \\
point finger at the other person & 80.16 & pat on back of other person   & 88.41 & 8.25 & pat on back of other person   \\
reach into pocket & 80.39 & eat meal/snack"   & 83.21 & 2.82 & wear on glasses   \\
drop & 80.45 & check time (from watch)   & 83.64 & 3.18 & sniff (smell)   \\
pat on back of other person & 81.25 & point finger at the other person   & 86.96 & 5.71 & point finger at the other person   \\
tear up paper & 82.03 & fold paper   & 86.35 & 4.32 & open a box   \\
whisper in other person’s ear & 82.13 & knock over other person (hit with body)   & 86.96 & 4.83 & knock over other person (hit with body)   \\
throw & 82.27 & tennis bat swing   & 88.00 & 5.73 & wear jacket   \\
brushing teeth & 82.52 & writing   & 89.01 & 6.49 & touch head (headache)   \\
% tennis bat swing & 82.62 & throw up cap/hat   & 78.75 & -3.88 & throw up cap/hat   \\
put on headphone & 82.96 & wear on glasses   & 87.52 & 4.57 & wear on glasses   \\
check time (from watch) & 83.42 & eat meal/snack"   & 89.49 & 6.07 & rub two hands together   \\
step on foot & 83.52 & kicking other person   & 86.26 & 2.74 & kicking other person   \\
\bottomrule 
\end{tabular}
}
\label{table:velocity_complete_action_imp_1}
\end{table*}

\begin{table*}[t]
% Second Half 
\caption{Velocity: Second Half. }
\resizebox{\textwidth}{!}{
\begin{tabular}{l|rc|rrc}
\toprule 
%\rowcolor{Gray}
 & \multicolumn{2}{c|}{\textbf{Joint}} & \multicolumn{3}{c}{\textbf{Concatenation: Joint + Angular}} \\
\cline{2-3}\cline{4-6}
%\rowcolor{Gray}
\multirow{-2}{*}{\textbf{Action}} & Acc (\%) & Similar Action & Acc (\%) & Acc$\uparrow$ (\%) & Similar Action \\ 
\midrule 
% \rowcolor{Gray!30}
grab other person’s stuff & 83.52 & wield knife towards other person   & 87.30 & 3.78 & touch other person's pocket   \\
toss a coin & 83.99 & thumb up   & 86.56 & 2.57 & snapping fingers   \\
brushing hair & 84.35 & brushing teeth   & 87.91 & 3.56 & use a fan (with hand or paper)/feeling warm   \\
shake head & 84.45 & typing on a keyboard   & 92.73 & 8.27 & touch neck (neckache)   \\
cross hands in front (say stop) & 84.51 & put the palms together   & 90.58 & 6.07 & put the palms together   \\
take a photo of other person & 84.59 & shoot at other person with a gun   & 90.10 & 5.51 & shoot at other person with a gun   \\
% apply cream on face & 85.06 & eat meal/snack"   & 81.71 & -3.36 & wipe face   \\
move heavy objects & 86.15 & carry something with other person   & 89.96 & 3.82 & carry something with other person   \\
take off bag & 86.15 & take off jacket   & 90.97 & 4.82 & take off jacket   \\
cheer up & 86.23 & hand waving   & 89.42 & 3.19 & use a fan (with hand or paper)/feeling warm   \\
use a fan (with hand or paper)/feeling warm & 86.27 & hand waving   & 88.36 & 2.09 & shake fist   \\
% rub two hands together & 86.32 & clapping   & 85.87 & -0.45 & clapping   \\
put on a hat/cap & 86.50 & wear on glasses   & 96.32 & 9.82 & wear on glasses   \\
punching/slapping other person & 86.59 & hit other person with something   & 86.86 & 0.27 & hit other person with something   \\
nod head/bow & 86.68 & touch chest (stomachache/heart pain)   & 94.93 & 8.25 & take off a shoe   \\
hand waving & 86.96 & use a fan (with hand or paper)/feeling warm   & 90.15 & 3.19 & use a fan (with hand or paper)/feeling warm   \\
% giving something to other person & 87.04 & exchange things with other person   & 86.23 & -0.81 & exchange things with other person   \\
touch back (backache) & 87.41 & touch chest (stomachache/heart pain)   & 91.30 & 3.90 & touch chest (stomachache/heart pain)   \\
put on bag & 87.52 & take off jacket   & 93.22 & 5.70 & wear jacket   \\
exchange things with other person & 87.52 & giving something to other person   & 88.52 & 1.00 & giving something to other person   \\
salute & 87.77 & kicking something   & 90.22 & 2.45 & brushing teeth   \\
cross toe touch & 87.85 & move heavy objects   & 89.37 & 1.52 & move heavy objects   \\
wear on glasses & 88.01 & eat meal/snack"   & 92.67 & 4.66 & brushing hair   \\
hands up (both hands) & 88.72 & stretch oneself   & 91.29 & 2.57 & stretch oneself   \\
touch chest (stomachache/heart pain) & 89.22 & touch back (backache)   & 90.22 & 1.00 & touch back (backache)   \\
touch other person's pocket & 89.55 & pat on back of other person   & 93.82 & 4.27 & giving something to other person   \\
put the palms together & 89.58 & check time (from watch)   & 90.94 & 1.36 & cross hands in front (say stop)   \\
cross arms & 90.13 & cross hands in front (say stop)   & 94.43 & 4.30 & put the palms together   \\
kicking other person & 90.30 & kicking something   & 91.30 & 1.00 & punching/slapping other person   \\
take off glasses & 90.97 & wear on glasses   & 92.70 & 1.73 & take off headphone   \\
pickup & 91.00 & take off a shoe   & 93.82 & 2.82 & take off a shoe   \\
hopping (one foot jumping) & 91.36 & running on the spot   & 96.73 & 5.36 & staggering   \\
juggling table tennis balls & 91.50 & open a box   & 94.42 & 2.92 & open a box   \\
pushing other person & 91.75 & punching/slapping other person   & 93.84 & 2.09 & touch other person's pocket   \\
bounce ball & 91.98 & juggling table tennis balls   & 93.51 & 1.53 & finger-guessing game (playing rock-paper-scissors)   \\
% stretch oneself & 92.23 & taking a selfie   & 91.15 & -1.08 & hands up (both hands)   \\
side kick & 92.55 & kicking something   & 94.95 & 2.39 & kicking something   \\
high-five & 92.58 & finger-guessing game (playing rock-paper-scissors)   & 95.66 & 3.08 & make victory sign   \\
carry something with other person & 92.75 & support somebody with hand   & 94.44 & 1.69 & support somebody with hand   \\
sitting down & 92.77 & falling   & 93.04 & 0.27 & nod head/bow   \\
butt kicks (kick backward) & 93.08 & side kick   & 95.30 & 2.22 & side kick   \\
% finger-guessing game (playing rock-paper-scissors) & 93.10 & use a fan (with hand or paper)/feeling warm   & 92.36 & -0.74 & use a fan (with hand or paper)/feeling warm   \\
handshaking & 93.20 & hugging other person   & 95.65 & 2.45 & pat on back of other person   \\
wear jacket & 93.55 & take off jacket   & 97.09 & 3.55 & take off jacket   \\
take off a hat/cap & 93.87 & take off glasses   & 95.24 & 1.37 & shake head   \\
% walking apart from each other & 94.29 & walking towards each other   & 93.84 & -0.45 & walking towards each other   \\
% follow other person & 94.49 & walking apart from each other   & 93.92 & -0.56 & walking apart from each other   \\
falling & 94.64 & squat down   & 97.09 & 2.45 & staggering   \\
squat down & 94.82 & sitting down   & 96.86 & 2.05 & sitting down   \\
jump up & 95.38 & running on the spot   & 98.19 & 2.81 & hopping (one foot jumping)   \\
% kicking something & 96.10 & standing up (from sitting position)   & 94.93 & -1.17 & side kick   \\
cheers and drink & 96.22 & grab other person’s stuff   & 97.39 & 1.17 & high-five   \\
% walking towards each other & 96.44 & walking apart from each other   & 94.14 & -2.30 & walking apart from each other   \\
staggering & 96.46 & kicking something   & 97.83 & 1.36 & walking towards each other   \\
running on the spot & 96.74 & bounce ball   & 97.04 & 0.30 & hopping (one foot jumping)   \\
hugging other person & 96.81 & check time (from watch)   & 98.18 & 1.36 & check time (from watch)   \\
arm swings & 96.91 & arm circles   & 97.91 & 1.00 & arm circles   \\
arm circles & 97.43 & stretch oneself   & 98.78 & 1.35 & stretch oneself   \\
% take off jacket & 97.55 & wear jacket   & 97.10 & -0.45 & wear jacket   \\
% standing up (from sitting position) & 97.90 & wear a shoe   & 96.34 & -1.56 & wear a shoe   \\
\bottomrule 
\end{tabular}
}
\label{table:velocity_complete_action_imp_2}
\end{table*}
